# Supplementary material for: EDLaaS: Fully Homomorphic Encryption Over Neural Network Graphs for Vision and Private Strawberry Yield Forecasting
Source: arXiv:2110.13638 source file (2022-10-18)
Supplement: Supplementary file 1 [file appendix.tex]

\begin{figure}[h]
  \centering
  \includegraphics[width=0.8\columnwidth]{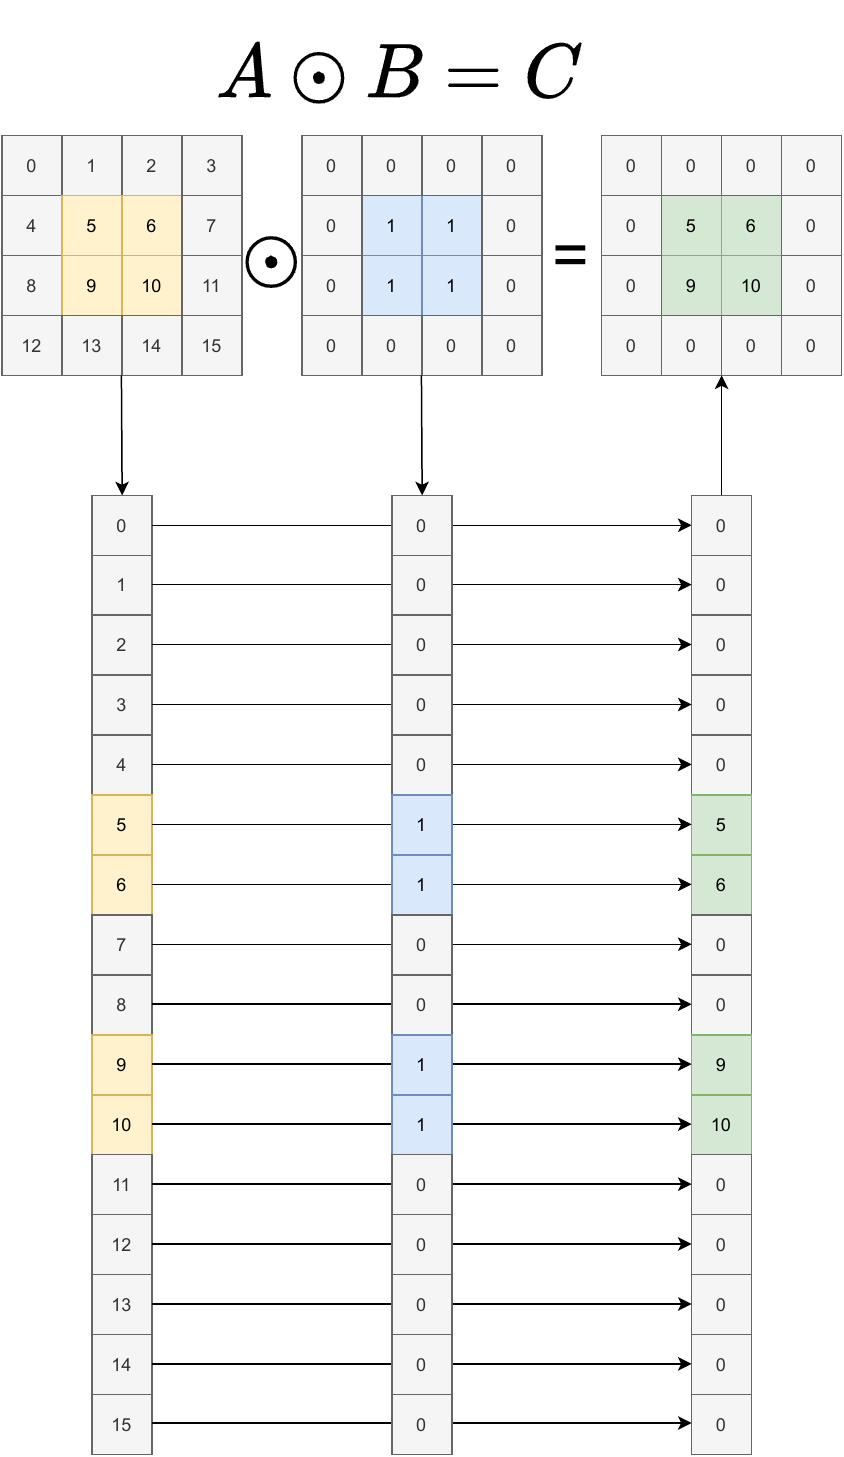}
  \caption{Hadmard product calculation depiction of two equally shaped matrices A and B, this is equivalent to vector products in arbitrary dimensions which is a core operation of our implementation since the shape of the cyphertext is the most atomic shape we can utilize without decrypting. \autocite{reseal}}
  \label{fig:hadmard_product}
\end{figure}
